# Supplementary material for: D$^2$iT: Dynamic Diffusion Transformer for Accurate Image Generation
Source: arXiv:2504.09454 source file (2025-04-13)
Supplement: Supplementary file 1 [file X_suppl.tex]

% \clearpage
\setcounter{page}{1}
\maketitle
% \maketitlesupplementary

\section{Detailed Implementations}
\label{sec:Detailed}
\textbf{Architectures of DVAE \& D$^2$iT.} In the first stage, DVAE follows the official implementation of VAE except for the proposed Dynamic Grained Coding module. For the hierarchical encoder, we add two residual blocks followed by a downsampling block to extract each feature map.

\begin{table}[t]
\centering
 \resizebox{\columnwidth}{!}{%
\begin{tabular}{@{}lcccc}
\toprule
Method & Layers & Patch size & Param(M) & FLOPs(G) \\ \hline
\multicolumn{5}{@{}l}{Network configurations of \textbf{Base}(B) models.} \\ 
DiT & 12 & 2 & 130 & 23.01 \\ 
DiT & 12 & 1 & 130 & 87.07 \\ 
\textbf{D$^2$iT}(Ours) & 10+2 & 2 \& 1 & 136 & \textbf{35.93} \\ \hline
\multicolumn{5}{@{}l}{Network configurations of \textbf{Large}(L) models.} \\
DiT & 24 & 2 & 458 & 80.71 \\ 
DiT & 24 & 1 & 457 & 309.51 \\ 
\textbf{D$^2$iT}(Ours) & 20+4 & 2 \& 1 & 467 & \textbf{102.25} \\ \hline
\multicolumn{5}{@{}l}{Network configurations of \textbf{Extra Large}(XL) models.} \\ 
DiT & 28 & 2 & 675 & 118.64 \\ 
DiT & 28 & 1 & 674 & 456.98 \\ 
\textbf{D$^2$iT}(Ours) & 22+6 & 2 \& 1 & 687 & \textbf{145.60} \\ \hline
% \multicolumn{5}{l}{Network configurations of DG-DiT models.} \\ \hline
% B & 10+2 & 2 \& 1 & 136 & 35.93 \\ \hline
% L & 22+2 & 2 \& 1 & 467 & 102.25 \\ \hline
% XL & 26+2 & 2 \& 1 & 687 & 145.60 \\ \hline
% \multicolumn{5}{l}{Network configurations of DiT baselines.} \\ \hline
% B & 12 & 2 & 130 & 23.01 \\ \hline
% L & 24 & 2 & 458 & 80.71 \\ \hline
% XL & 28 & 2 & 675 & 118.64 \\ \hline
% B & 12 & 1 & 130 & 87.07 \\ \hline
% L & 24 & 1 & 457 & 309.51 \\ \hline
% XL & 28 & 1 & 674 & 456.98 \\ \hline
\end{tabular}    }
\caption{Comparison of network configurations of D$^2$iT and DiT. The number of D$^2$iT layers consists of DiT Backbone and Efficient RefineNet. FLOPs are measured with a latent embedding size of 32$\times$32$\times$4. }
\label{Comparison_of_network}
\end{table}

\begin{figure*}[t]
  \centering
   \includegraphics[width=1\linewidth]{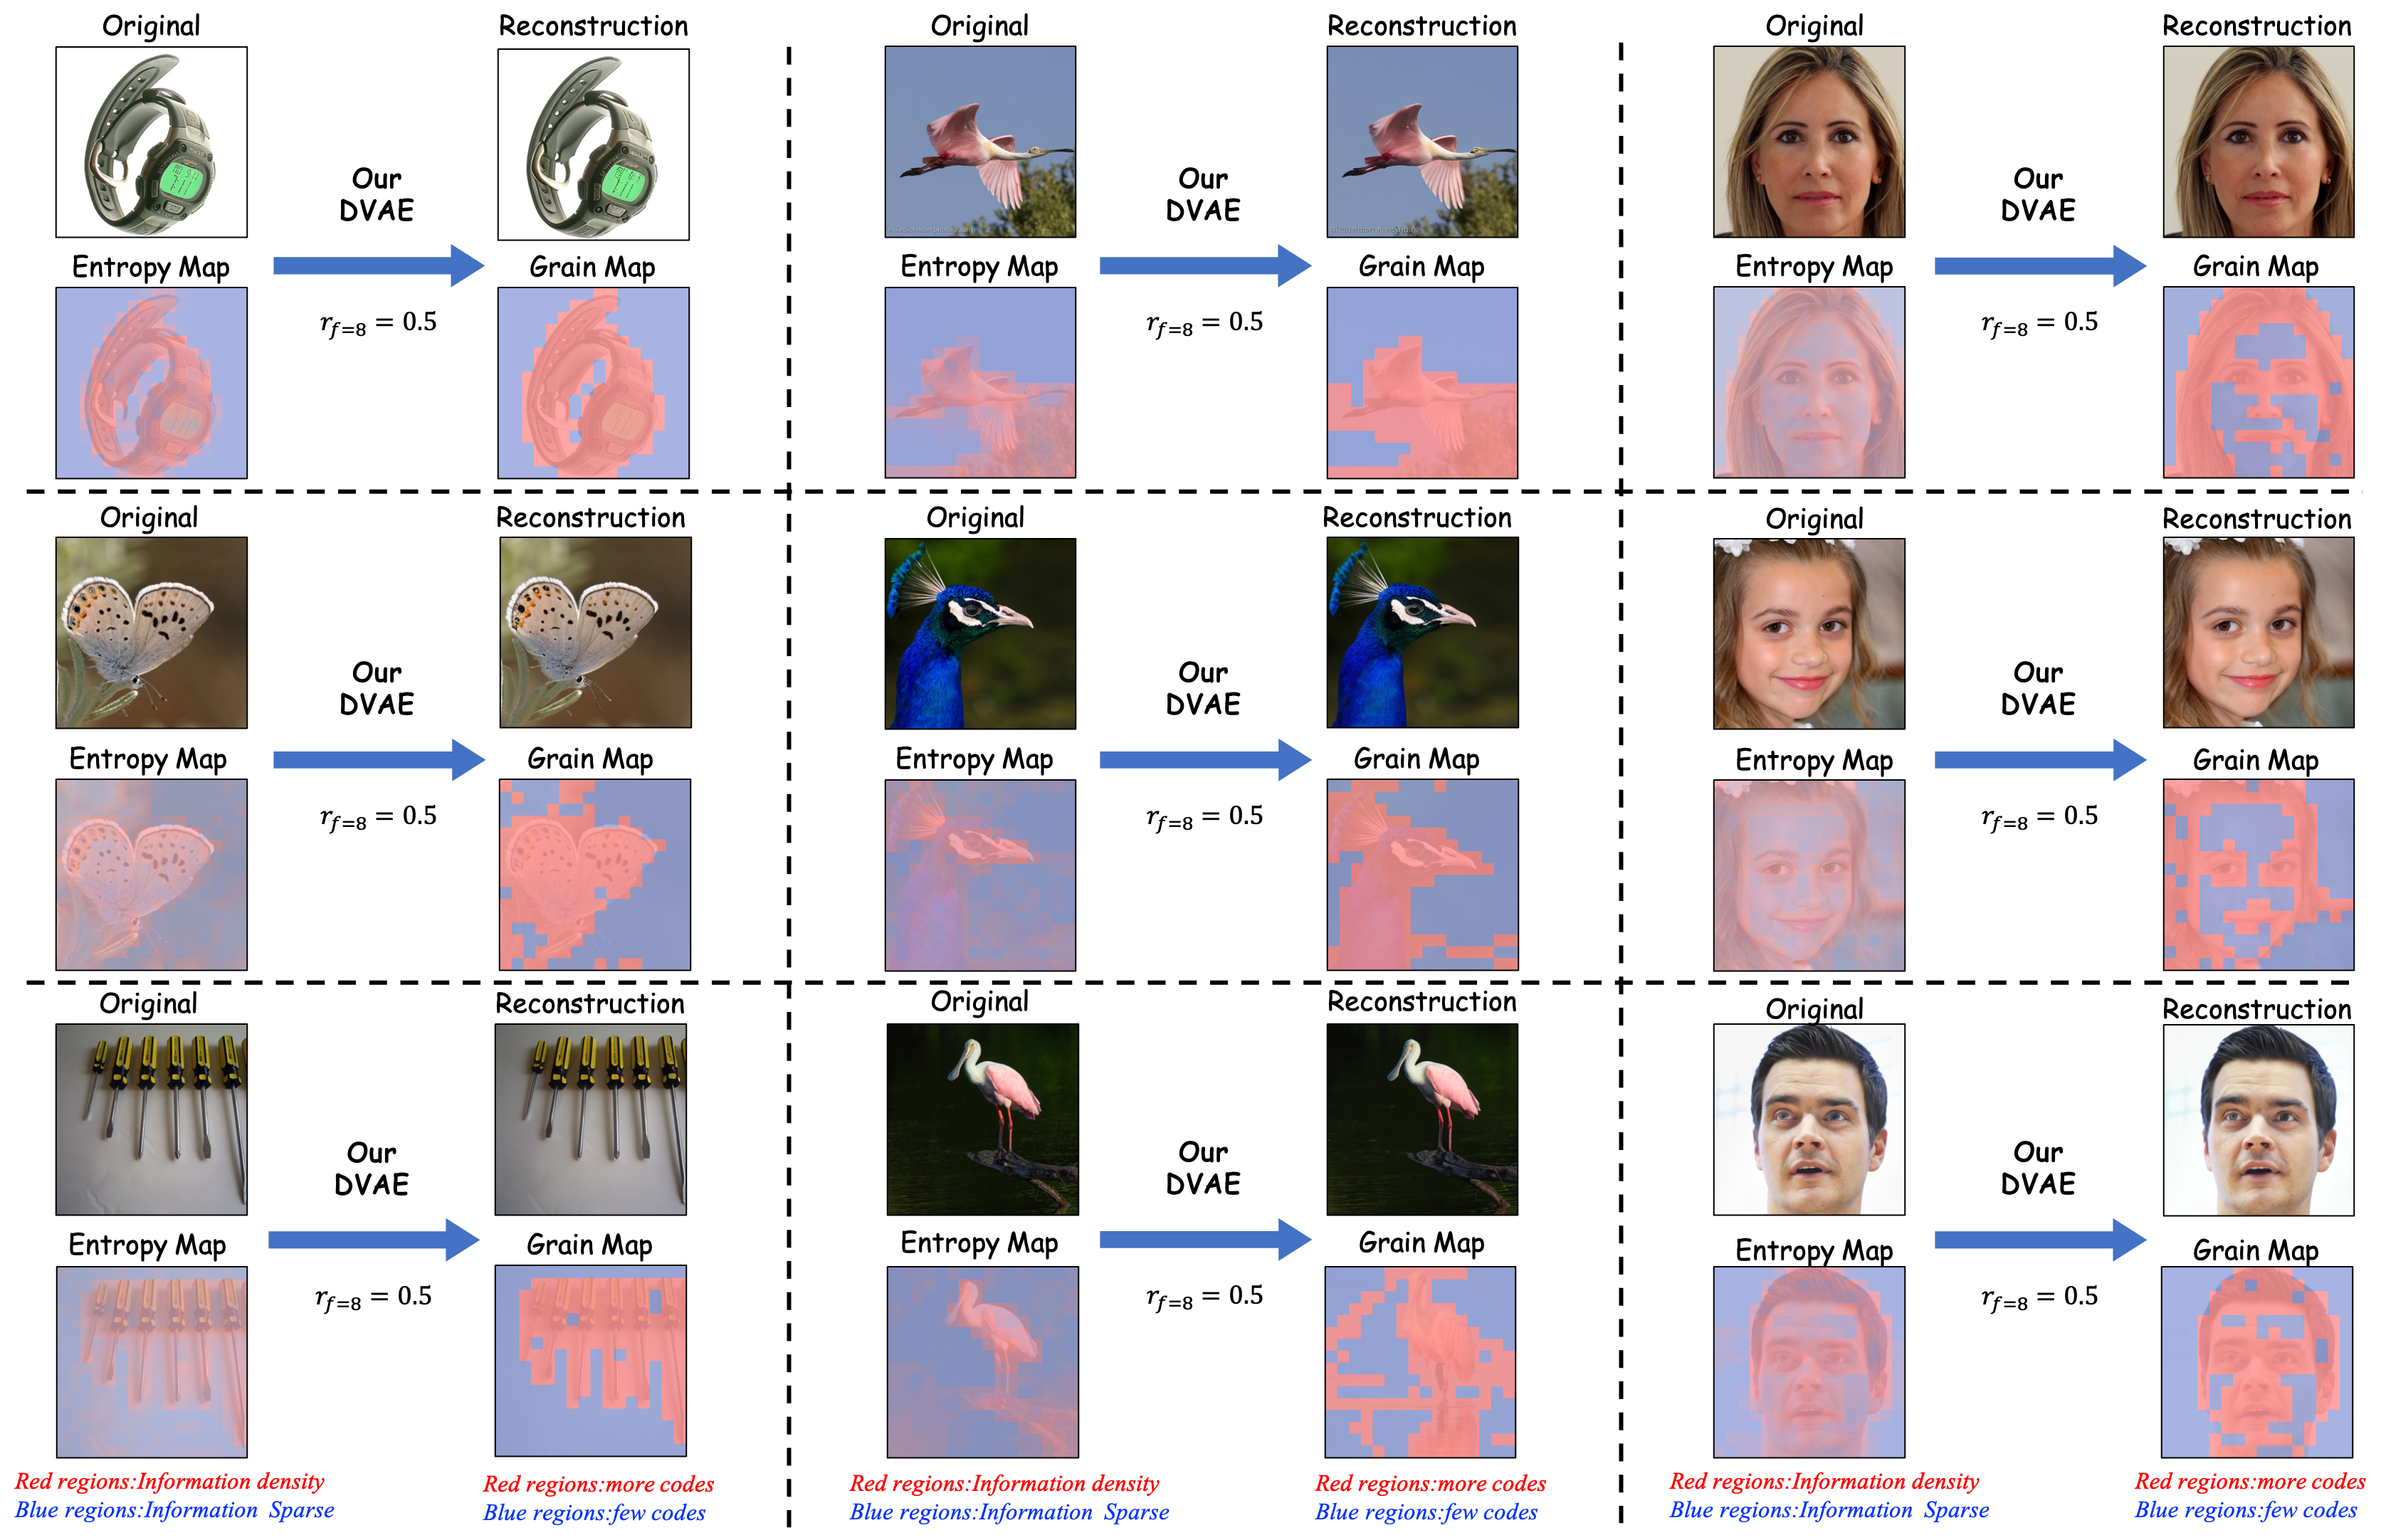}

   \caption{Visualization of the variable-length coding of our DVAE, where our grain map exactly matches the entropy map of the original image and therefore leads to more accurate and natural coding representations, \textit{i.e.}, the \textcolor{red}{information-dense regions} in entropy map are more red and deserves \textcolor{red}{more latent codes} to reduce the reconstruction error, while  \textcolor{blue}{information-sparse regions} where VAE has lower reconstruction error are assigned \textcolor{blue}{few latent codes}.}
   \label{fig:vis_first_stage}
\end{figure*}

\begin{table}[t]
  \centering
     \resizebox{\columnwidth}{!}{%
\begin{tabular}{lccc}
\toprule
Model  & D$^2$iT-B  & D$^2$iT-L  & D$^2$iT-XL    \\
\hline
Parameters & 136M & 467M & 687M   \\
Flops & 35.93G & 102.25G & 145.60G  \\
\hline
Coarse Grain & $16\times 16\times 4$ & $16\times 16\times 4$ & $16\times 16\times 4$  \\
Fine Grain & $32\times 32\times 4$ & $32\times 32\times 4$ & $32\times 32\times 4$  \\
Total Layers & 12 & 24 & 28  \\ \midrule
\textbf{DiT backbone} &  &  & \\ 
\quad Patch size & 2 & 2 & 2  \\
\quad Layers & 10 & 20 & 22  \\
\quad Dimensions & 768 & 1024 & 1152  \\
\quad Heads & 12 & 16 & 16  \\ \midrule
\textbf{RefineNet} &  &   &    \\
\quad Patch size & 1 & 1 & 1 \\
\quad  Layers & 2 & 4 & 6  \\
\quad Dimensions & 768 & 1024 & 1152 \\
\quad Window size & $16\times 16$ & $16\times 16$& $16\times 16$\\
\hline
Batch size & 256 & 256 & 256  \\
Optimizer & AdamW & AdamW & AdamW \\
learning rate & $1\times 10^{-4}$ & $1\times 10^{-4}$ & $1\times 10^{-4}$ \\
\hline
Sampler  &  DDPM  &   DDPM  &  DDPM   \\
Sampling steps &250 &250 &250 \\
\bottomrule
\end{tabular}}
\caption{Experimental setup of Dynamic Content Transformer of D$^2$iT with different parameters.}
\label{experimental_setup}
\end{table}

\begin{table}[ht]
\centering
\fontsize{9}{10}\selectfont % 设置字体为 
\begin{tabular}{ccc}
\toprule
regularization &  DVAE rFID-10K$\downarrow$ & D$^2$iT-B FID-10K$\downarrow$ \\
\midrule
\textit{VQ-reg.}  & 2.38 & 25.23\\
\textit{KL-reg.}  & 2.09 & 22.11\\
\bottomrule
\end{tabular}
\caption{Ablations of regularization for reconstruction of DVAE and generation of D$^2$iT-B on FFHQ.}
\label{vq_KL_DGVAE}
\end{table}

In the second stage, we use the same adaLN-Zero settings as DiT to modify RefineNet Blocks. Table \ref{Comparison_of_network} shows the parameter count and Gflops of D$^2$iT compared to DiT\cite{peebles2023scalable}. More  details and experimental training settings at different model sizes of the Dynamic Content Transformer in D$^2$iT
 are listed in Table \ref{experimental_setup}. In addition, the probability of dropout is all set to be 0.1 for all layers. And we set the total number of the Dynamic Content Transformer layers (\ie, DiT backbone  + RefineNet) according to DiT, achieving base-, large-, and extra large-sized models, denoted by D$^2$iT-B/L/XL. The Gflops of D$^2$iT are significantly smaller than those of the DiT model with the patch size set to 1.

\textbf{Training Details.} DVAE is trained with Adam optimizer with $\beta_1 = 0.5$ and $\beta_2 = 0.9$, and the base learning rate is set at $4.5 \times 10^{-6}$ following  \cite{rombach2022high}. The weight for adversarial loss is set to be 0.75 and the weight for perceptual loss is set to be 1.0. For FFHQ, DVAE is trained for 80 epochs with a linear learning rate warmed up during the first epoch. For ImageNet, DVAE is trained for 50 epochs with a linear learning rate warmed up during the first 0.5 epochs. 

The Dynamic Grain Transformer (predict grain map) and Dynamic Content Transformer (predict multi-grained noise) of D$^2$iT are trained using AdamW optimizer with parameters $\beta_1 = 0.9$ and $\beta_2 = 0.999$. The weight decay is set to be 0.01. We use a constant learning rate of $1 \times 10^{-4}$, and utilize DDPM Sampler with 250 steps like previous works. The training batch size is 256, and there is no weight decay. In the main experiment, D$^2$iT-L and D$^2$iT-XL are trained for 800 epochs for FFHQ and ImageNet. In the ablation experiments, D$^2$iT-B is trained for 50 epochs for FFHQ. 

\section{More Analysis of DVAE}

\subsection{Impact of regularization \textit{\textbf{VQ-reg.}} \& \textit{\textbf{KL-reg.}}}
We experiment with two different types of regularizations.
The first variant, \textit{KL-reg.}, imposes a slight KL-penalty towards a standard normal on the learned latent, similar to a VAE, as used in  \cite{peebles2023scalable}, whereas \textit{VQ-reg.} incorporates a vector quantization
layer within the decoder, similar to a VQGAN in  \cite{esser2021taming}. As shown in Table \ref{vq_KL_DGVAE}, we conduct ablation studies on the FFHQ benchmark, testing DVAE with dual granularities $F = {8, 16}$ and a fine-grained ratio $r_{f =8} = 0.5$, to assess its effect on image generation in D$^2$iT. The \textit{VQ-reg.} is trained with codebook size $K = 1024$. And all of the models are trained for 50 epochs. The \textit{KL-reg.} regularization shows better performance in reconstruction quality for the first stage, and it provides a latent representation that is easier to learn for the second stage of image generation. \textit{KL-reg.} provides a latent representation of a continuous space that is more suitable for D$^2$iT than \textit{VQ-reg.}

\subsection{More Visualization}

We provide more visualization of our information-density-based dynamic latent coding in Figure \ref{fig:vis_first_stage}. The output of DVAE contains Multi-grained latent code and the corresponding grain map.  We show that the grain map matches image entropy map for both simple and complex regions, \textit{i.e.}, important regions are assigned more codes and unimportant ones are assigned few codes, leading to more sensible reconstruction.

\section{More Analysis of D$^2$iT}
\subsection{Impact of the Window size of RefineNet.} 
The windows of RefineNet are arranged to evenly partition the image in a non-overlapping manner. Supposing each window contains $M \times M$ patches, the computational complexity of a global multi-head self attention(MSA) module and a window-based one on an image of $h \times w$ patches are:
\begin{equation}
\Omega(\text{MSA}) = 4hwC^2 + 2(hw)^2C,
  \label{eq:complexity}
\end{equation}

\begin{equation}
\Omega(\text{W-MSA}) = 4hwC^2 + 2(M)^2hwC,
  \label{eq:complexity}
\end{equation}
where the former MSA of standard Transformer is quadratic to patch number $h\times w$, and the latter W-MSA of RefineNet Transformer is linear when $M$ is fixed. 

\begin{figure*}[t]
  \centering
   \includegraphics[width=1\linewidth]{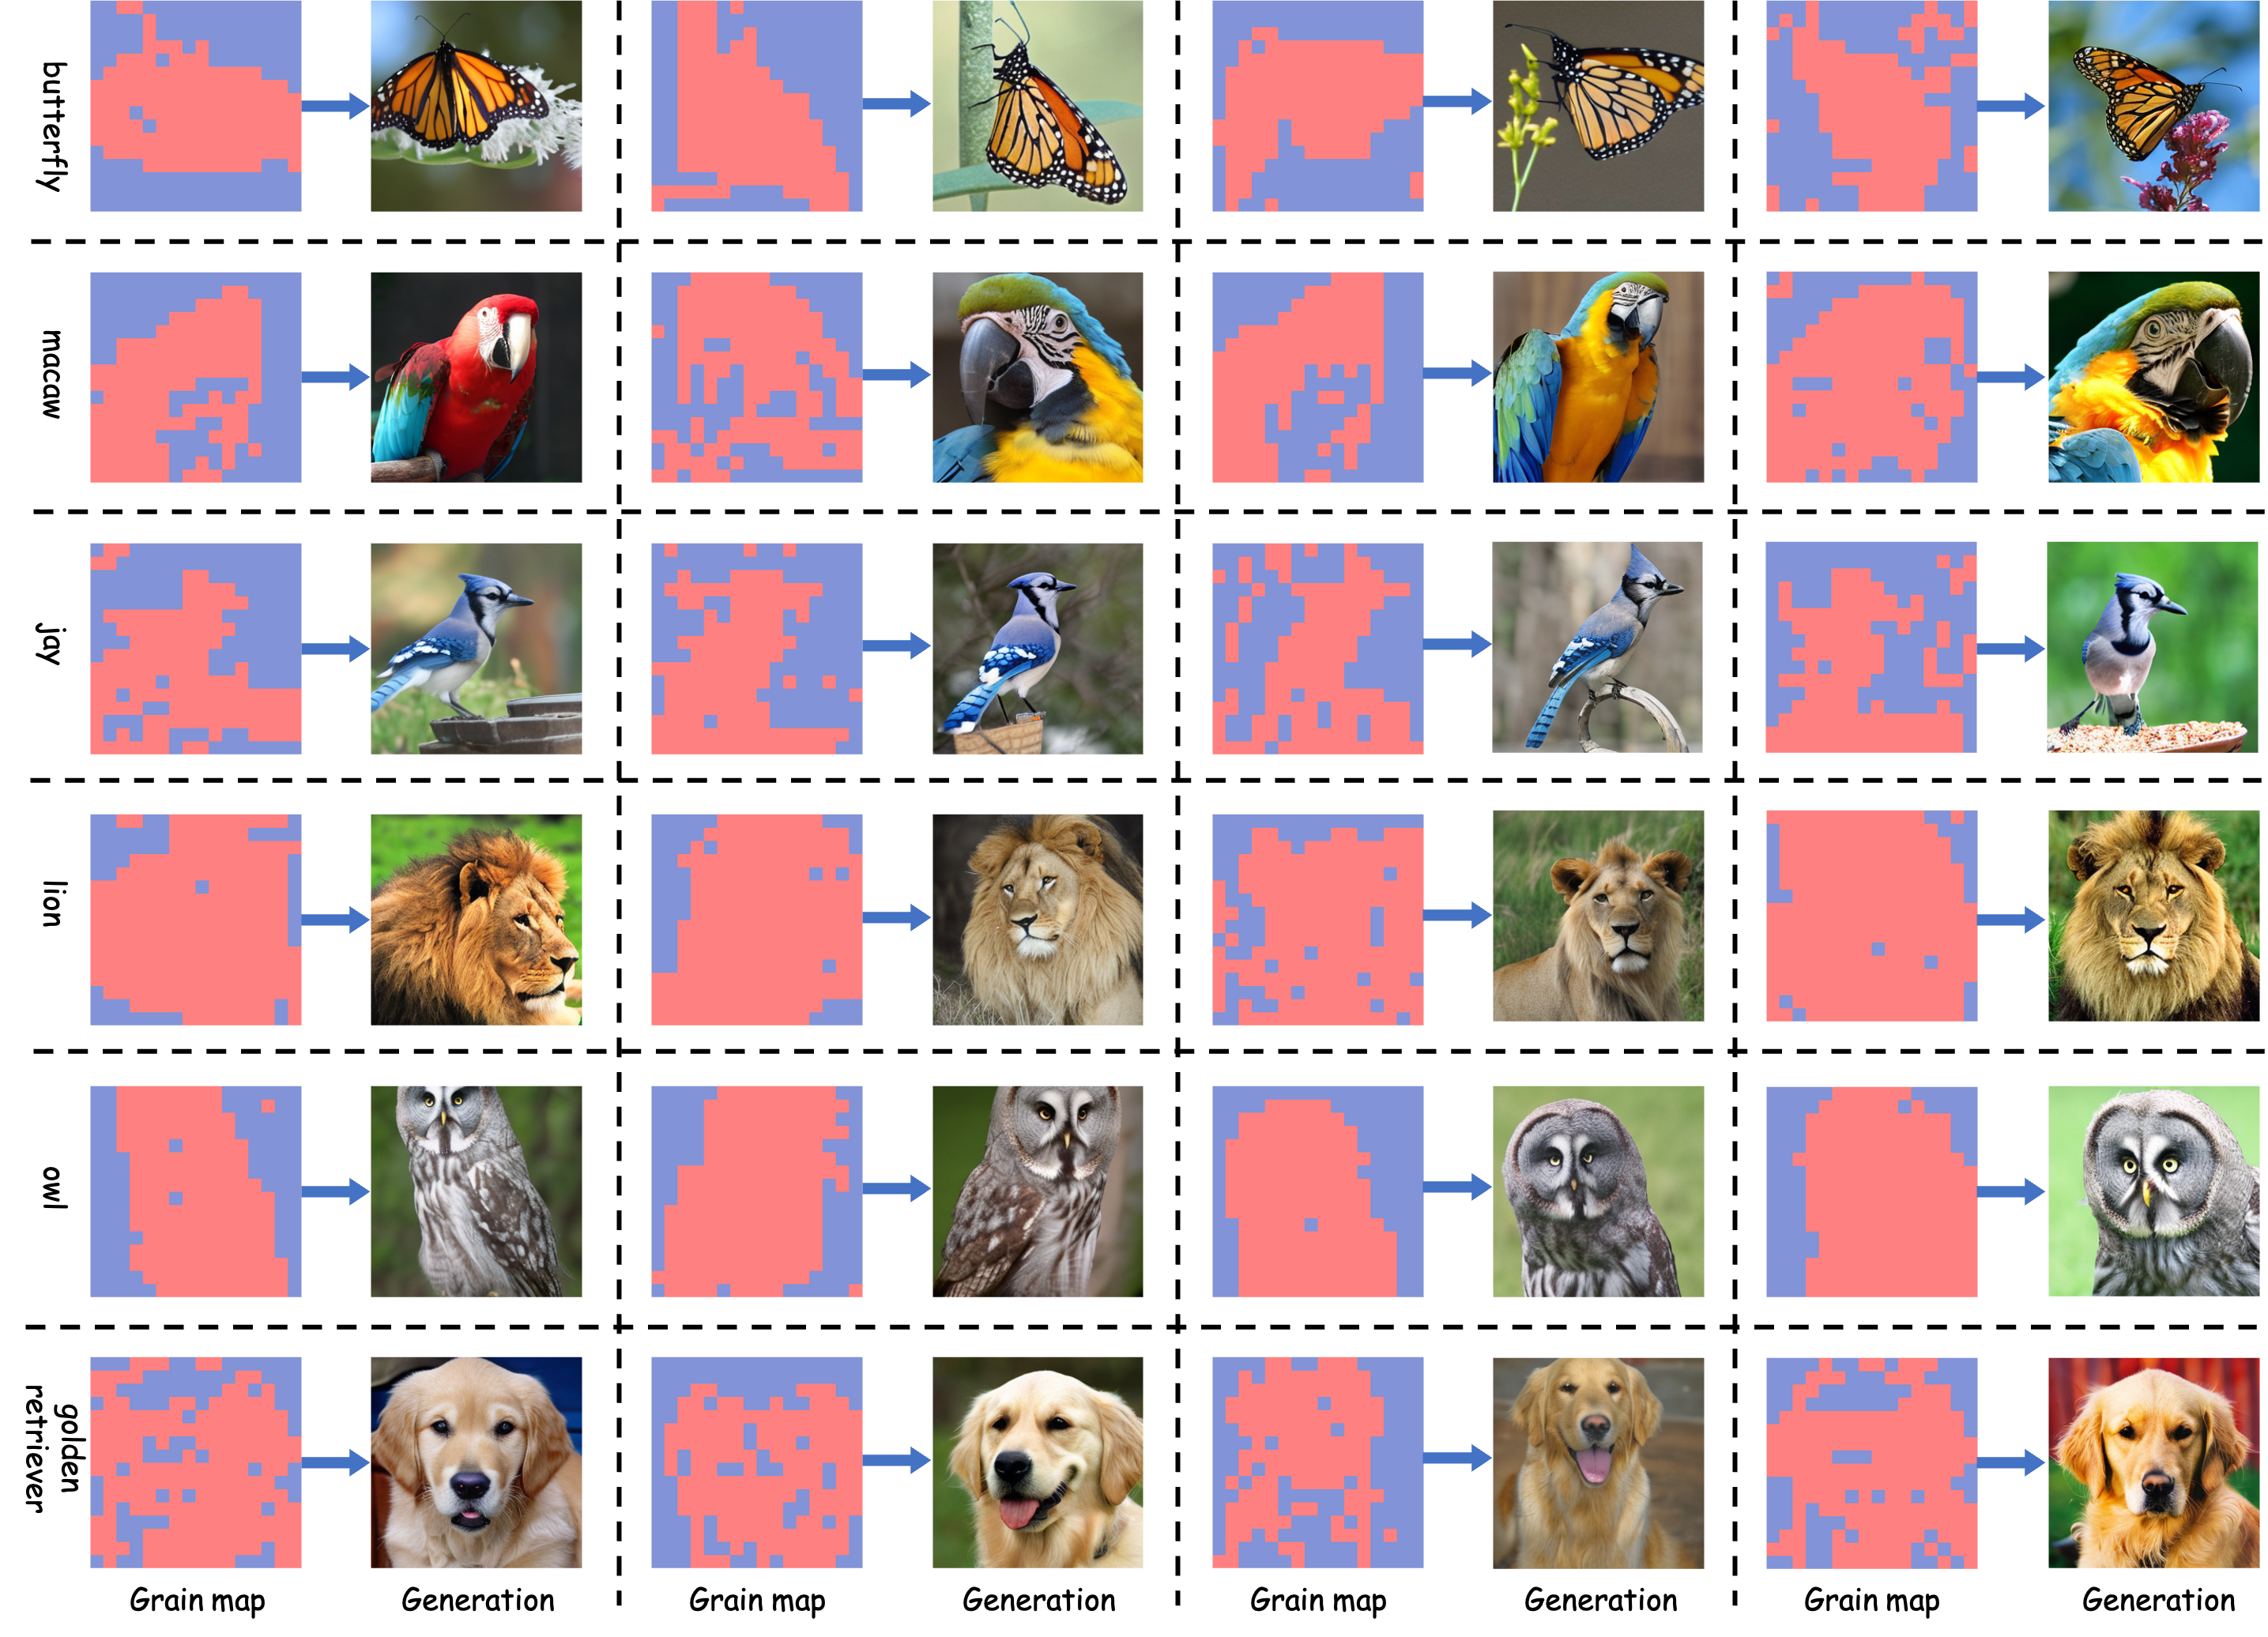}

   \caption{Visualization of the grain map \& generation image with D$^2$iT-XL on ImageNet. The grain map size is 16$\times$16, with red indicating fine-grained regions (codes with 8$\times$ downsampling) and blue indicating coarse-grained regions (codes with 16$\times$ downsampling).}
   \label{fig:vis_generation}
\end{figure*}

We compared the effect of different window sizes in Table \ref{dit_window_size}. 
We observe that images generated using RefineNet are significantly better than those using the DiT backbone alone, further demonstrating the need for fine-grained noise corrections. When the window size varies, the generation FID scores differ slightly, with the model performing best when the window size is set to 16. Thus, we conclude that for $32\times 32\times 4$ hidden spaces, the optimal window size is 16 for the best performance.

\begin{table}[t]
\centering
\fontsize{9}{10}\selectfont % 设置字体为 
\begin{tabular}{cc}
\toprule
Window size &  FID-10K$\downarrow$  \\
\midrule
w/o & 27.62 \\
16  & 22.11 \\
8  & 23.56 \\
4 & 23.82 \\
2 & 23.93 \\
\bottomrule
\end{tabular}
\caption{Effect of window size for RefineNet of D$^2$iT-B on FFHQ.}
\label{dit_window_size}
\end{table}

\begin{table}[t]
\centering
\fontsize{9}{10}\selectfont % 设置字体为 8pt，行距为 10pt
\begin{tabular}{lc}
\toprule
 Grain Map Setting & FID-50K$\downarrow$ \\
\midrule
Random &  12.65 \\ %
Ground Truth & 1.70  \\
Dynamic Grain Transformer & 1.73 \\
\bottomrule
\end{tabular}
\caption{Effect of Dynamic Grain Transformer with D$^2$iT-XL on ImageNet.}
\label{DGT_ablation_imagenet}
\end{table}

\begin{figure*}[t]
  \centering
   \includegraphics[width=1\linewidth]{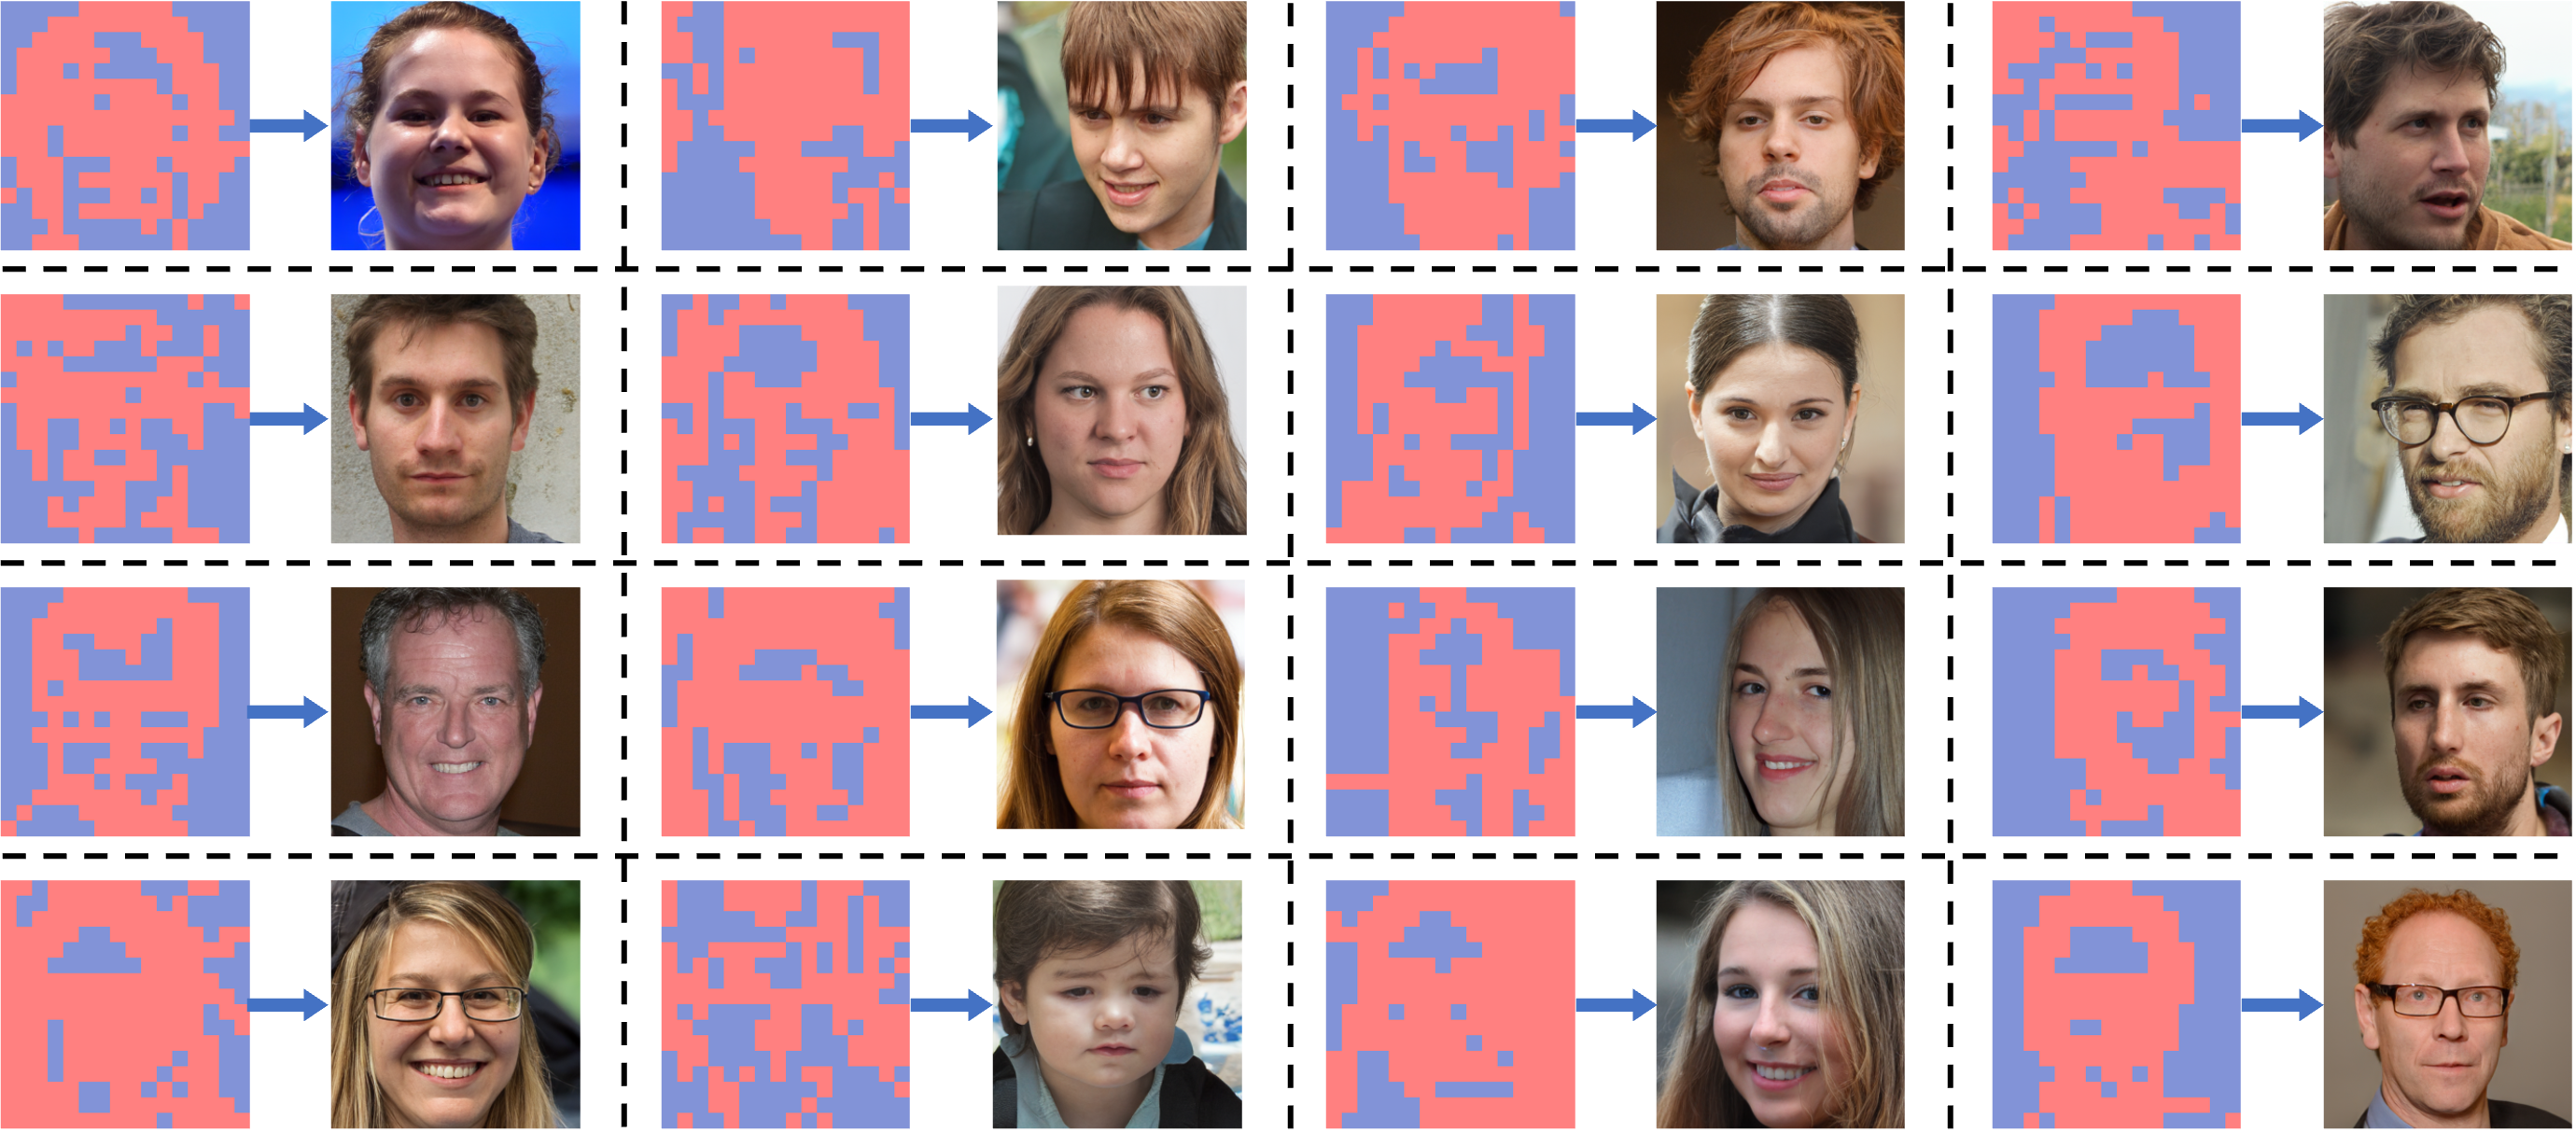}

   \caption{Visualization of the grain map \& generation image with D$^2$iT-L on FFHQ.}
   \label{fig:vis_generation_ffhq}
\end{figure*}

\subsection{Impact of the Dynamic Grain Transformer.} 

In the ablation experiment described in the main text, we demonstrate the impact of the grain map generated by the Dynamic Grain Transformer in D$^2$iT-L on the images generated under FFHQ. Here, we complement this by showing the impact of the grain map generated by the Dynamic Grain Transformer in D$^2$iT-XL under ImageNet on class-conditionally generated images. The results of grain maps generated by the Dynamic Grain Transformer are comparable to the ground truth grain maps of the ImageNet dataset and significantly better than random grain maps, \ie, the generated grain map with an FID score of 1.73 versus the ground truth grain map with an FID score of 1.70. This demonstrates that the Dynamic Grain Transformer can effectively model the spatial distribution of different classes in ImageNet.

\subsection{More Visualization}

More examples of D$^2$iT-XL’s generated results on ImageNet can be found in Figure \ref{fig:vis_generation}, and D$^2$iT-L’s generated results on FFHQ are shown in Figure \ref{fig:vis_generation_ffhq}. For different generated grain maps, D$^2$iT can generate a variety of images. This indicates that D$^2$iT achieves a diverse global representation. At the same time, the information density distribution of the generated image complies well with the grain map. This demonstrates that the Dynamic Content Transformer can capture the global structure, thereby more effectively constructing images that conform to the spatial density distribution specified by the grain map.
